# Supplementary material for: InfraParis: A multi-modal and multi-task autonomous driving dataset
Source: arXiv:2309.15751 source file (2023-11-06)
Supplement: Supplementary file 1 [file paper_supp.tex]

% % WACV 2024 Paper Template
% % based on the CVPR 2023 template (https://media.icml.cc/Conferences/CVPR2023/cvpr2023-author_kit-v1_1-1.zip) with 2-track changes from the WACV 2023 template (https://github.com/wacv-pcs/WACV-2023-Author-Kit)
% % based on the CVPR template provided by Ming-Ming Cheng (https://github.com/MCG-NKU/CVPR_Template)
% % modified and extended by Stefan Roth (stefan.roth@NOSPAMtu-darmstadt.de)

% \documentclass[10pt,twocolumn,letterpaper]{article}

% %%%%%%%%% PAPER TYPE  - PLEASE UPDATE FOR FINAL VERSION
% %\usepackage[review,algorithms]{wacv}      % To produce the REVIEW version for the algorithms track
% %\usepackage[review,applications]{wacv}      % To produce the REVIEW version for the applications track
% \usepackage{wacv}              % To produce the CAMERA-READY version
% %\usepackage[pagenumbers]{wacv} % To force page numbers, e.g. for an arXiv version

% % Include other packages here, before hyperref.
% \usepackage{graphicx}
% \usepackage{amsmath}
% \usepackage{amssymb}
% \usepackage{booktabs}
% \usepackage{multirow}
% \usepackage{makecell}
% \usepackage{rotating}
% \usepackage{tabularray}
% \usepackage{diagbox}

% \usepackage{bm}
% \usepackage{adjustbox}
% \usepackage{array}
% \usepackage{pifont}
% \usepackage{float}
% \usepackage{xfrac}
% \usepackage{colortbl}
%     \usepackage[normalem]{ulem}
% \usepackage{mathtools}
% \usepackage{breqn}
% \usepackage{stmaryrd}

% \usepackage{caption}
% \usepackage{subcaption}

% \usepackage{comment}
% \usepackage[dvipsnames,table]{xcolor}
% \usepackage{soul}
% \usepackage{cite}


% \newcommand\gianni{\textcolor{red}}
% \newcommand\marwane{\textcolor{blue}}
% \newcommand\nacim{\textcolor{RoyalBlue}}
% \newcommand\xuanlong{\textcolor{purple}}
% \definecolor{forestgreen}{rgb}{0.13, 0.55, 0.13}
% \newcommand\antoine{\textcolor{forestgreen}}
% \newcommand\david{\textcolor{orange}}

% \input{abbrev.tex}

% % It is strongly recommended to use hyperref, especially for the review version.
% % hyperref with option pagebackref eases the reviewers' job.
% % Please disable hyperref *only* if you encounter grave issues, e.g. with the
% % file validation for the camera-ready version.
% %
% % If you comment hyperref and then uncomment it, you should delete
% % ReviewTempalte.aux before re-running LaTeX.
% % (Or just hit 'q' on the first LaTeX run, let it finish, and you
% %  should be clear).
% \usepackage[pagebackref,breaklinks,colorlinks]{hyperref}


% % Support for easy cross-referencing
% \usepackage[capitalize]{cleveref}
% \crefname{section}{Sec.}{Secs.}
% \Crefname{section}{Section}{Sections}
% \Crefname{table}{Table}{Tables}
% \crefname{table}{Tab.}{Tabs.}



% %%%%%%%%% PAPER ID  - PLEASE UPDATE
% \def\wacvPaperID{1319} % *** Enter the WACV Paper ID here
% \def\confName{WACV}
% \def\confYear{2024}


% \begin{document}

% %%%%%%%%% TITLE - PLEASE UPDATE
% \title{InfraParis: A multi-modal and multi-task autonomous driving dataset \\------ Supplementary material ------}

% \author{Gianni Franchi\\
% U2IS, ENSTA Paris, IP Paris\\
% {\tt\small gianni.franchi@ensta-paris.fr}
% \and
% Marwane Hariat\\
% U2IS, ENSTA Paris, IP Paris\\
% {\tt\small marwane.hariat@ensta-paris.fr}
% \and
% Xuanlong Yu\\
% SATIE, Paris-Saclay University; 
% U2IS, ENSTA Paris, IP Paris\\
% {\tt\small xuanlong.yu@ensta-paris.fr}
% \and
% Nacim Belkhir\\
% Safrantech, Safran Group\\
% {\tt\small nacim.belkhir@safrangroup.com}
% \and
% Antoine Manzanera\\
% U2IS, ENSTA Paris, IP Paris\\
% {\tt\small antoine.manzanera@ensta-paris.fr}
% \and
% David Filliat\\
% U2IS, ENSTA Paris, IP Paris\\
% {\tt\small david.filliat@ensta-paris.fr}
% }


% \maketitle


% \appendix
% \renewcommand{\theequation}{A\arabic{equation}}
% \renewcommand{\thetable}{A\arabic{table}}
% \renewcommand{\thefigure}{A\arabic{figure}}

% % \setcounter{equation}{4}
% % \setcounter{figure}{2}
% % \setcounter{table}{4}


% %%%%%%%%% BODY TEXT
% \input{supplementary}


% \end{document}
